# Supplementary material for: Tunable symmetry breaking and helical edge transport in a graphene quantum spin Hall state
Source: arXiv:1307.5104 source file (2013-07-19)

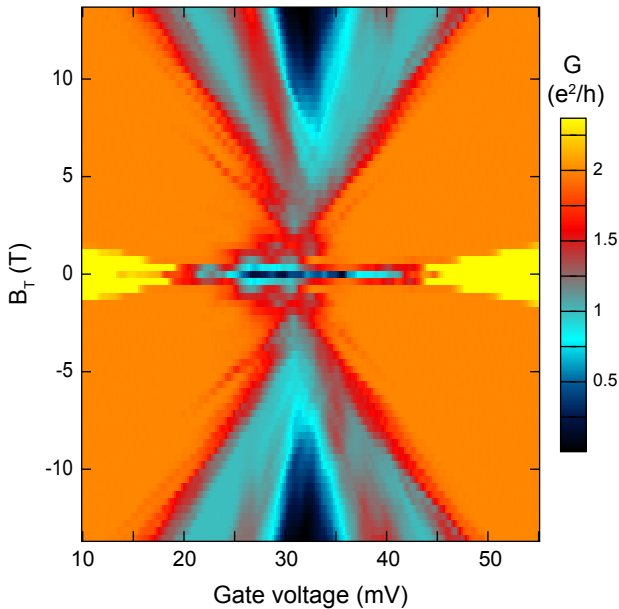

Supplement: Supplementary file 1 [file suppfig-colorplotbigms5.pdf]
